# Supplementary material for: BOCO: Bayesian Online Contextual Optimization for Decision-Focused Online Learning
Source: arXiv:2511.20413 source file (2026-09-23)
Supplement: Supplementary file 1 [file supplement.tex]

\documentclass[twoside]{article}

\usepackage[preprint]{aistats2026}
\usepackage[colorlinks=true,    % Enable colored links
            linkcolor=blue,     % For internal links (sections, etc.)
            citecolor=blue,     % For citation links
            urlcolor=blue       % For URLs
]{hyperref}
\usepackage{mathtools}
\usepackage{amsfonts}
\usepackage{amsmath}
\usepackage{mathrsfs}
\usepackage{amsthm}
\newtheorem{theorem}{Theorem}
 % Theorem A, B, C, ...

\newtheorem{corollary}{Corollary}
 % Use letters instead of numbers

\newcommand{\bm}{\boldsymbol}
\newcommand{\condi}{\mathcal{F}_{t-1},x_t}
\newcommand{\lra}[1]{\left(#1\right)}
\newcommand{\lrb}[1]{\left[#1\right]}

% If your paper is accepted, change the options for the package
% aistats2026 as follows:
%
%\usepackage[accepted]{aistats2026}
%
% This option will print headings for the title of your paper and
% headings for the authors names, plus a copyright note at the end of
% the first column of the first page.

% If you set papersize explicitly, activate the following three lines:
%\special{papersize = 8.5in, 11in}
%\setlength{\pdfpageheight}{11in}
%\setlength{\pdfpagewidth}{8.5in}

% If you use natbib package, activate the following three lines:
\usepackage[round]{natbib}

% If you use BibTeX in apalike style, activate the following line:
%\bibliographystyle{apalike}

\begin{document}

% If your paper is accepted and the title of your paper is very long,
% the style will print as headings an error message. Use the following
% command to supply a shorter title of your paper so that it can be
% used as headings.
%
\runningtitle{PAC-Bayes Online Contextual Optimization}

% If your paper is accepted and the number of authors is large, the
% style will print as headings an error message. Use the following
% command to supply a shorter version of the authors names so that
% they can be used as headings (for example, use only the surnames)
%
%\runningauthor{Surname 1, Surname 2, Surname 3, ...., Surname n}

% Supplementary material: To improve readability, you must use a single-column format for the supplementary material.
\onecolumn
\aistatstitle{PAC-Bayes Meets Online Contextual Optimization: \\ Supplementary Materials}

\section{MISSING PROOFS}
\subsection{Proofs of Theorem 3.2 and 3.3}
Theorems 3.2 and 3.3 are direct results of Corollary 3.1 and Corollary 3.3 from~\cite{PACBonline} with modifications on (i) the condition in the conditional distribution of $\boldsymbol{\xi}_t$, and (ii) the constant term in the bound. We start by presenting the original Corollary 3.1 in \cite{PACBonline} and Theorem 3.2 in this work using our notation.

\begin{corollary}[\cite{PACBonline}, Corollary 3.1]
Suppose Assumption 3.1 holds. For any distribution $\mu$ over $D$, any $\lambda > 0$, any $\delta \in (0,1)$, and any online posterior $\{\tilde{\pi}\}$ and prior $\{\pi\}$ sequences, the following inequality holds with at least probability $1 - \delta$ over the draw $D \sim \mu$:
\begin{equation*}
    \sum_{t=1}^{T} \mathbb{E}_{\theta \sim \tilde{\pi}_{t+1}}[\mathbb{E}[\ell(\theta, d_t)|\mathcal{F}_{t-1}]] \\
    \leq\sum_{t=1}^{T} \left( \mathbb{E}_{\theta \sim \tilde{\pi}_{t+1}}[\ell(\theta, d_t)] + \frac{\mathbb{D}_{KL}(\tilde{\pi}_{t+1}\Vert\pi_t)}{\lambda} \right) \\
    + \frac{\lambda TC^2}{2} + \frac{\log(1/\delta)}{\lambda} .
\end{equation*}
\end{corollary}
\setcounter{theorem}{1}
\begin{theorem}\label{T32}
Suppose Assumption 3.1 holds. For any distribution $\mu$ over $D$, any $\lambda > 0$, any $\delta \in (0,1)$, and any online posterior $\{\tilde{\pi}\}$ and prior $\{\pi\}$ sequences, the following inequality holds with at least probability $1 - \delta$ over the draw $D \sim \mu$:
\begin{equation*}
    \sum_{t=1}^{T} \mathbb{E}_{\theta \sim \tilde{\pi}_{t+1}}[\mathbb{E}[\ell(\theta, \boldsymbol{\xi}_t)|\mathcal{F}_{t-1},x_t]] 
    \leq\sum_{t=1}^{T} \left( \mathbb{E}_{\theta \sim \tilde{\pi}_{t+1}}[\ell(\theta, d_t)] + \frac{\mathbb{D}_{KL}(\tilde{\pi}_{t+1}\Vert\pi_t)}{\lambda} \right) 
    + \frac{\lambda TC^2}{8} + \frac{\log(1/\delta)}{\lambda} .
\end{equation*}
\end{theorem}
The first difference lies between $\mathbb{E}[\ell(\theta,d_t)|\mathcal{F}_{t-1}]$ and $\mathbb{E}[\ell(\theta, \boldsymbol{\xi}_t)|\mathcal{F}_{t-1},x_t]$ in the l.h.s.. The second difference lies in the denominator for the term $\lambda T C^2$.

For the first difference, since $x_t$ has already been realized, it is $\mathcal{F}_{t-1}$-measurable. Therefore, by the tower probability and measurability of $x_t$, for all $\theta$ we can write:
\begin{equation}
    \mathbb{E}_{(X_t=x_t,\boldsymbol{\xi}_t)}[\ell(\theta,(X_t=x_t, \boldsymbol{\xi}_t))|\mathcal{F}_{t-1}] = \mathbb{E}_{X_t}[  \mathbb{E}_{\boldsymbol{\xi}_t}[\ell(\theta, \boldsymbol{\xi}_t)|\mathcal{F}_{t-1}, X_t=x_t] |\mathcal{F}_{t-1}] \label{e1}\tag{A.1}
\end{equation}
Because $X_t = x_t$ is observed, $\mathbb{P}\{X_t=x_t|\mathcal{F}_{t-1},x_t\} = 1$. Thus, the outer expectation $\mathbb{E}_{X_t}[\cdot|\mathcal{F}_{t-1}]$ in the r.h.s.~of Eq~\eqref{e1} degenerates to the form in Theorem~\ref{T32}. Note that if the target risk $\mathbb{E}_{(X_t,\boldsymbol{\xi}_t)}[\ell(\theta, (X_t,\boldsymbol{\xi}_t))|\mathcal{F}_{t-1}]$ is adopted, it suggests that we also have to predict/estimate the covariate $x_t$ for the next step, which differs from the setting of contextual optimization.

The second difference is due to the modification of the bound range in Hoeffding's lemma. According to Assumption 3.1, we know the loss $\ell(\theta,d_t) \in [0,C], \forall \theta, \forall d_t$, while \cite{PACBonline} considered the range $[-C,C]$. Therefore, $\forall \theta, \forall d_t$,
\begin{equation*}
    \Delta_t(\theta) = \mathbb{E}[\ell(\theta,\boldsymbol{\xi}_t)|\mathcal{F}_{t-1},x_t] - \ell(\theta, d_t) \in [\mu(\theta,x_t,\mathcal{F}_{t-1}) - C, \mu(\theta,x_t,\mathcal{F}_{t-1})],
\end{equation*}
where $\mu(\theta,x_t,\mathcal{F}_{t-1})$ is a constant (expectation) for a given $(x_t, \theta, \mathcal{F}_{t-1})$. Therefore, Hoeffding's lemma applies as follows:
\begin{equation*}
    \mathbb{E}[e^{ \lambda \Delta_t(\theta)}|\mathcal{F}_{t-1},x_t] \leq e^{\lambda^2 C^2 / 8}.
\end{equation*}
Applying this inequality in Lemma D.2 in~\cite{PACBonline} and keeping other proofs unchanged will give Theorem 3.2. Similarly, Corollary 3.3 in~\cite{PACBonline} can be modified in the same way.
\subsection{Proof of Corollary 3.5}
\proof
By Assumption 3.4, we have $\forall \lambda > 0, \forall d \in \mathcal{X} \times \Xi, \forall \pi \in \mathcal{P}(\Xi)$:
\begin{equation}
    \ell\lra{\pi,d} \leq -\frac{1}{\lambda} \log \mathbb{E}_{\theta \sim \pi}\lrb{e^{-\lambda \ell(\theta,d)}}  \label{e1}\tag{A.1}
\end{equation}
In other words, this assumption ensures the pseudo-likelihood $e^{-\lambda \ell(\pi,d)}$ when implementing a decision optimized for posterior $\pi$ is always better than the expected pseudo-likelihood $e^{-\lambda \ell(\theta,d)}$ of an individual drawn $\theta \sim \pi$. We leverage this assumption to bound the risk of the aggregated predictor based on the risk of the stochastic predictor.

Applying the convexity of $e^x$ in $x$ point-wise for $d$ gives:
\begin{equation}
     \mathbb{E}_{\theta \sim \pi}\lrb{e^{-\lambda \ell\lra{\theta,d}}} \geq e^{-\lambda \mathbb{E}_{\theta \sim \pi}\lrb{\ell\lra{\theta,d}}} \label{e2}\tag{A.2}.
\end{equation}
Taking Eq~\eqref{e2} into Eq~\eqref{e1} gives:
\begin{equation}
     \ell\lra{\pi,d}  \leq -\frac{1}{\lambda} \log \lra{
     \mathbb{E}_{\theta \sim \pi}\lrb{
     e^{-\lambda \ell\lra{\theta,d}}
     }
     } \leq -\frac{1}{\lambda}\log\left(
     e^{-\lambda \mathbb{E}_{\theta \sim \pi}\lrb{\ell(\theta,d)}}
     \right) = \mathbb{E}_{\theta \sim \pi}\lrb{\ell(\theta,d)}. \label{e3}\tag{A.3}
\end{equation}
Here, Eq~\eqref{e3} is very similar to the direct application of convexity of $\ell$ in $\theta$ if one regards the $\pi$ as the mean $\mathbb{E}_{\theta \sim \pi}[m(x;\theta)]$. However, because we input the pushforward distribution into decision-making rather than the posterior mean, we thus leverage the mixability of $\ell$ to circumvent the requirement of convexity.

Taking expectation $\mathbb{E}\lrb{\cdot|\mathcal{F}_{t-1},x_t}$ on both sides of Eq~\eqref{e3} gives:
\begin{equation}
    \mathbb{E}\lrb{\ell\lra{\pi,\bm{\xi}_t}|\condi} \leq \mathbb{E}\lrb{
    \mathbb{E}_{\theta \sim \pi}\lrb{
    \ell\lra{\theta,\bm{\xi}_t}
    }|\condi
    } \label{e4}\tag{A.4}.
\end{equation}
Finally, by the measurability of $\pi_t$ given $\mathcal{F}_{t-1}$ and Fubini's theorem, the expectation in the r.h.s.~of Eq~\eqref{e4} can be swapped as:
\begin{equation}
    \mathbb{E}\lrb{\ell\lra{\pi,\bm{\xi}_t}|\condi} \leq 
    \mathbb{E}_{\theta \sim \pi}\lrb{
    \mathbb{E}\lrb{
    \ell\lra{\theta,\bm{\xi}_t}|\condi
    }
    }\label{e5}\tag{A.5},
\end{equation}
which holds almost surely and independently of the draw of data $D \sim \mu$. Applying this upper bound in Eq~\eqref{e5} to the l.h.s.~of Theorem 3.3 finishes the proof.

\endproof
\section{EXPERIMENTAL DETAILS}
The code of the experiments will be available soon. For all experiments, we use the open-source package \texttt{SCIPY}~\citep{scipy} to solve the deterministic and chance-constrained MILP problems.
\subsection{Data Generation and Hypothesis}
Our data generation follows the ARMA(2,2) process proposed in~\cite{wsaa} to construct a time-series $(x_t,\xi_t)$. Specifically, for each stage $t$:
\begin{equation*}
x_t = u_t + \Phi_1 x_{t-1} + \Phi_2 x_{t-2} + \Theta_1 u_{t-1} + \Theta_2 u_{t-2},
\end{equation*}
where $u_t \sim \mathcal{N}(\bm{0}, \Sigma_U)$ are innovations, and all the matrices are chosen as:
\begin{align*}
    \Phi_1 = \begin{bmatrix}
        0.5 & -0.9 & 0.0 \\
        1.1 & -0.7 & 0.0 \\
        0.0 & 0.0  & 0.5
    \end{bmatrix}, \quad
    \Phi_2 = \begin{bmatrix}
        0.0 & -0.5 & 0.0 \\
        -0.5 & 0.0 & 0.0 \\
        0.0 & 0.0  & 0.0
    \end{bmatrix},
\end{align*}
\begin{align*}
    \Theta_{1}=
    \begin{bmatrix}
    0.4 & 0.8 & 0.0 \\
    -1.1 & -0.3 & 0.0 \\
    0.0 & 0.0 & 0.0
    \end{bmatrix},
    \quad
    \Theta_{2}=
    \begin{bmatrix}
    0.0 & -0.8 & 0.0 \\
    -1.1 & 0.0 & 0.0 \\
    0.0 & 0.0 & 0.0
    \end{bmatrix},
    \quad
    \Sigma_{U}=
    \begin{bmatrix}
    1.0 & 0.5 & 0.0 \\
    0.5 & 1.2 & 0.5 \\
    0.0 & 0.5 & 0.8
    \end{bmatrix}.
\end{align*}
For each stage, once $x_t$ is generated, we generate the uncertainty $\xi_t$ as follows:
\begin{equation*}
    \tilde{\xi}_t = G (x_t + \delta_t / 4) + (B x_t)\circ \epsilon_t,
\end{equation*}
where $\delta_t$ and $\epsilon_t$ are independently sampled from standard Gaussian distribution, and matrices $G$ and $B$ are chosen as:
\begin{align*}
    G = 2.5 \times \begin{bmatrix}
        0.8 & 0.1 & 0.1 \\
        0.1 & 0.8 & 0.1 \\
        0.1 & 0.1 & 0.8 \\
        0.8 & 0.1 & 0.1 \\
        0.1 & 0.8 & 0.1 \\
        0.1 & 0.1 & 0.8 \\
        0.8 & 0.1 & 0.1 \\
        0.1 & 0.8 & 0.1 \\
        0.1 & 0.1 & 0.8 \\
        0.8 & 0.1 & 0.1 \\
        0.1 & 0.8 & 0.1 \\
        0.1 & 0.1 & 0.8
    \end{bmatrix}, \qquad 
    B = 7.5 \times \begin{bmatrix}
        0 & -1 & -1 \\
        -1 & 0 & -1 \\
        -1 & -1 & 0 \\
        0 & -1  & 1 \\
        -1 & 0 & 1 \\
        -1 & 1 & 0 \\
        0 & 1 & -1 \\
        1 & 0 & -1 \\
        1 & -1 & 0 \\
        0 & 1 & 1 \\
        1 & 0 & 1 \\
        1 & 1 & 0
    \end{bmatrix}.
\end{align*}
Having $\tilde{\xi}_t \in \mathbb{R}^{12}$, we do $\xi_{t,i} = \frac{\max\{-100, \tilde{\xi}_{t,i}\}}{100} + 2$ 
for each element in $\tilde{\xi}_t$ to ensure nonnegativity of weights. Eventually, we stack every 4 elements in the vector for a row, resulting in a matrix $A_t \in \mathbb{R}^{3 \times 4}$ as the weight matrix in optimization. 

We adopt an almost-linear model with a \texttt{sigmoid} activation function for the prediction task. Denote weights $W \in \mathbb{R}^{3 \times 12}$, bias $b \in \mathbb{R}^{12}$, and \texttt{sigmoid} function: $S(x) = \frac{1}{1 + e^{-x}}$. The forward prediction can be written as:
\begin{equation*}
    \hat{A}_t = 2S(W x_t + b),
\end{equation*}
while model parameter $\theta$ denotes the aggregation of weights and bias. We reshape the prediction to meet the dimension of the weight matrix. In total, the dimension of $\Theta$ is $ 3 \times 12 + 12 = 48$. 
\subsection{Framework Details}
\subsubsection{\texttt{BMA}}
In the implementation of \texttt{BMA} framework, we specify the following parameters: the initial prior $\pi_0 = \mathcal{N}(\bm{0}, I_{48})$, the shrinkage factor $a = 0.9$, the temperature $\lambda = 10^{-4}$, the Effective Sample Size threshold $\tau = 0.5$, the number of MCMC steps $L = 3$, the number of particles in SMC $N = 20$, the feasibility chance $\alpha = 0.9$. We choose relatively small $L$ and $N$ since we found they can already lead to satisfactory results while saving computational resources. Having all predictions $\hat{A}_t^i$ and the according weights $w_t^i$ for each prediction, we input these data in the following MILP problem to prescribe the decision $\hat{z}_t$ for each stage $t$ in the \texttt{BMA} framework under chance constraint:
\begin{align*}
    \max_{u, z, V, l} \quad & \sum_{i=1}^{N} w_t^i ( V^i + q^\top l^i)& \\
    \text{s.t.} \quad & \sum_{i=1}^{N} w_t^i u^i \geq \alpha \\
    & \hat{A}_t^i z \leq b + (1 - u^i)M, & i = 1, \cdots, N \\
    & 0 \leq V^i \leq u^i M, & i = 1, \cdots, N \\
    & V^i \geq c^\top z - ( 1- u^i) M, & i = 1, \cdots, N \\
    & l^i \leq b - \hat{A}^i_t z + M (1 - u^i), & i = 1, \cdots, N \\
    & l^i \geq b - \hat{A}^i_t z - M (1 - u^i), & i = 1, \cdots, N \\
    & 0 \leq l^i \leq u^i M,                    & i = 1, \cdots, N,\\
    & u \in \{0,1\}^{20}, z \in \mathbb{N}^4, V \in \mathbb{R}^{20}, l \in \mathbb{R}^{20 \times 3}.
\end{align*}
with $M$ here denotes a sufficiently large number to achieve the big-M modeling.
\subsubsection{\texttt{BGS}}
The \texttt{BGS} framework is a variant of \texttt{BMA}. Instead of leveraging the posterior approximation (by samples and weights) into the chance-constrained program for decision-making, \texttt{BGS} draws an indicator $I_t \sim \text{Cat}(w_t^1,\dots, w_t^N)$ to approximate the sampling from the posterior $\pi_t$, and input $\hat{A}_t^{I_t}$ into the deterministic program to prescribe a decision.
\subsubsection{\texttt{PtO}}
The \texttt{BGS} framework leverages online gradient descent (OGD) to minimize the MSE loss between the uncertainty realization $A_t$ and $\hat{A}_t$ predicted by a deterministic model. The model updated rule follows the classic OGD algorithm:
\begin{equation*}
    \theta_{t+1}^{pto} = \theta_{t}^{pto} - \eta_t\nabla_\theta \sqrt{\sum_i \sum_j (A_{t,i,j} - \hat{A}_{t,i,j})^2}.
\end{equation*}
Later, the updated model parameters will be used to predict the uncertainty $A_{t+1}$ for the next stage. In the experiments, we use standard Gaussian to initialize the parameters of \texttt{PtO} model. 

We use Adam optimizer to update the model parameters with a step decay step size of $0.99$. The initial learning rate is chosen as $0.1$ in our experiments, which is optimal in terms of MSE performance among $[0.01,0.05,0.1,0.5,1, 5, 10]$ for 20 trials with length $T = 500$. Figure~\ref{fig:sup1} demonstrates the time-averaged cumulative MSE loss within the \texttt{PtO} framework using different learning rates.

\begin{figure*}[!h]
    \centering
    \includegraphics[width=0.95\textwidth]{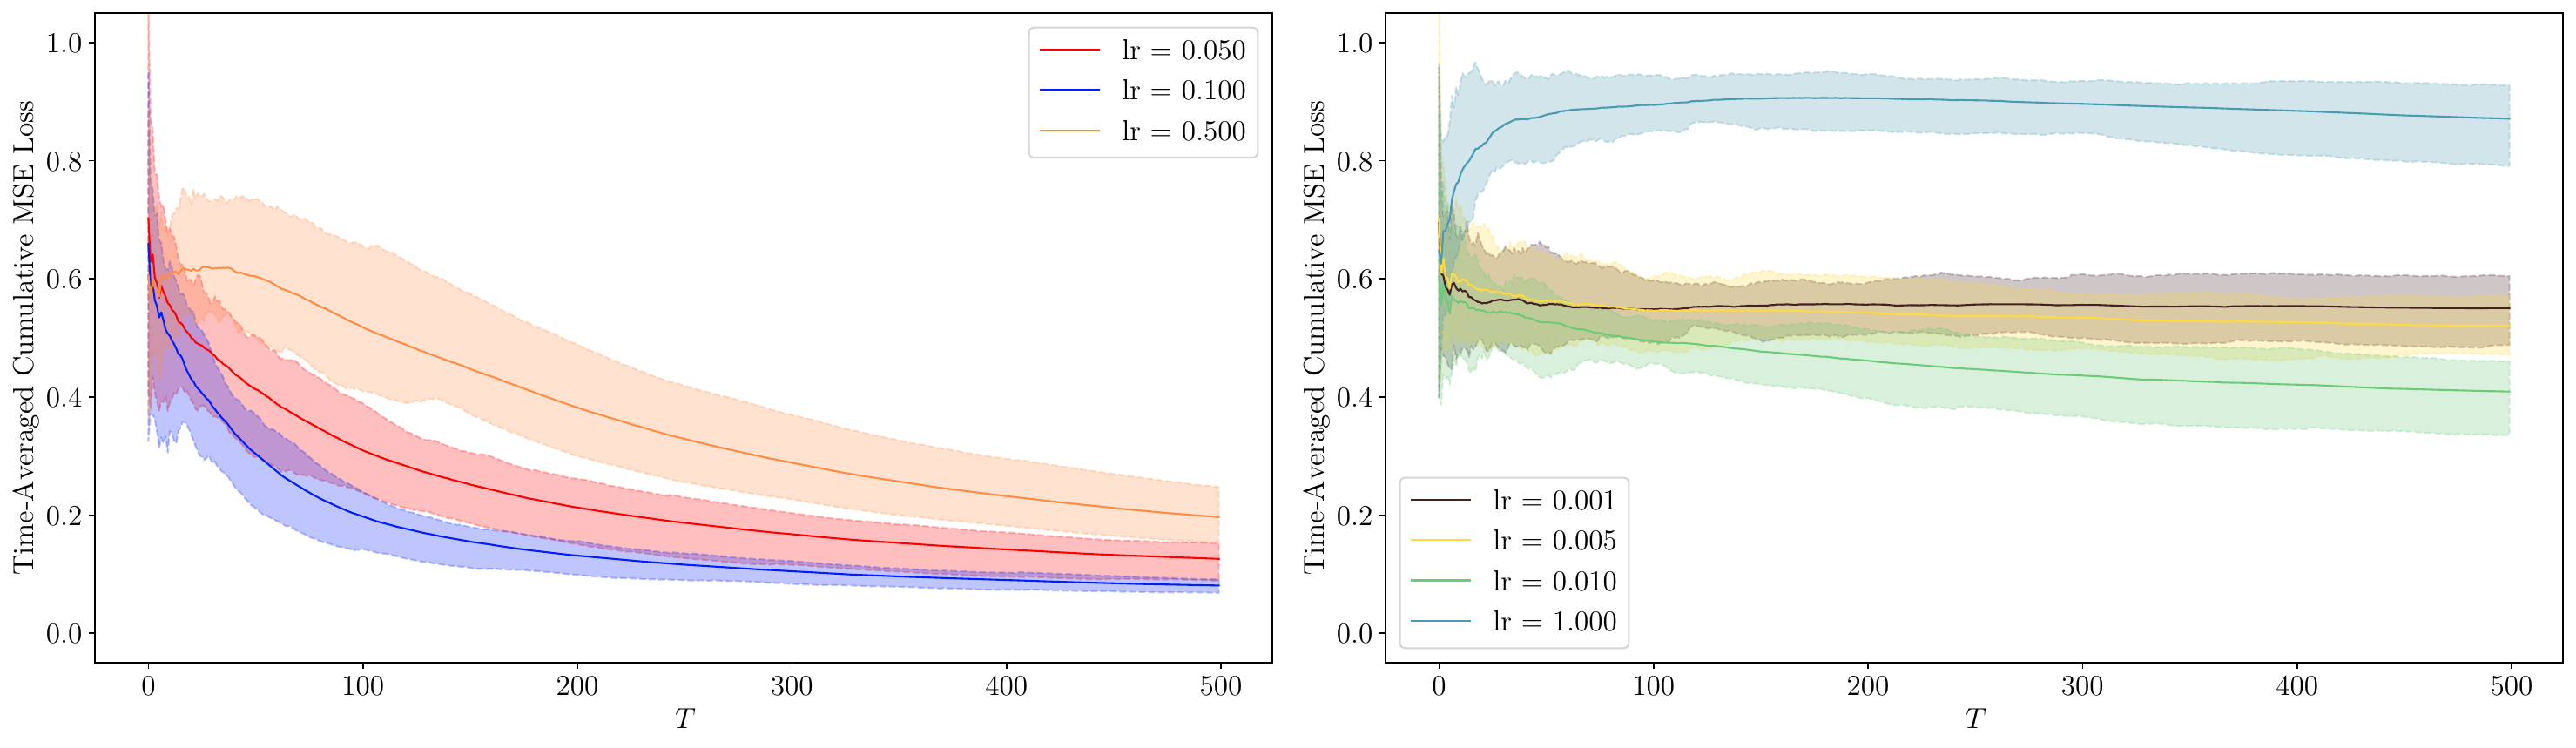}
    \caption{Time-averaged cumulative MSE loss for \texttt{PtO} with different learning rate. Results are computed from 20 trials with a horizon $T = 500$.}\label{fig:sup1}
\end{figure*}
\subsubsection{\texttt{DFL}}
The \texttt{DFL} framework leverages the gradient of the decision quality of the last stage to update the deterministic predictive model parameters. Because we consider an integer knapsack problem that is nondifferentiable, we approximate the gradient for \texttt{DFL} using score function gradient approximation. Consider at stage $t$, the \texttt{DFL} model prediction is $\hat{A}_t$ and uncertainty realization is $A_t$. To approximate the gradient of $\ell$ w.r.t. $\hat{A}_t$, we draw $K$ random noise $\{\epsilon^i\}$ from $\mathcal{N}(0, I_{\text{dim}(A_t)})$. Then, the gradient $\nabla_{A} \ell$ can be approximated as:
\begin{equation*}
    \nabla_A \ell \approx \frac{1}{K} \sum_{i=1}^{K} \lra{c'(\textbf{P}(\hat{A}_t + \epsilon^i), A_t) - \min_{z} c(z;A_t)}
    \epsilon^i.
\end{equation*}
In this work, we take $K = 20$ to match the computational cost of \texttt{BMA} in each update. The optimizer and step decay schedule are the same as \texttt{PtO}. $0.1$ is chosen as he initial learning rate for \texttt{DFL}, which is optimal in terms of average reward among $[0.001,0.005,0.01,0.05,0.1,0.5,1]$ for 20 trials with length $T = 500$. Figure~\ref{fig:sup2} demonstrates the time-averaged cumulative reward for \texttt{DFL} using different learning rates.
\begin{figure*}[!h]
    \centering
    \includegraphics[width=.95\textwidth]{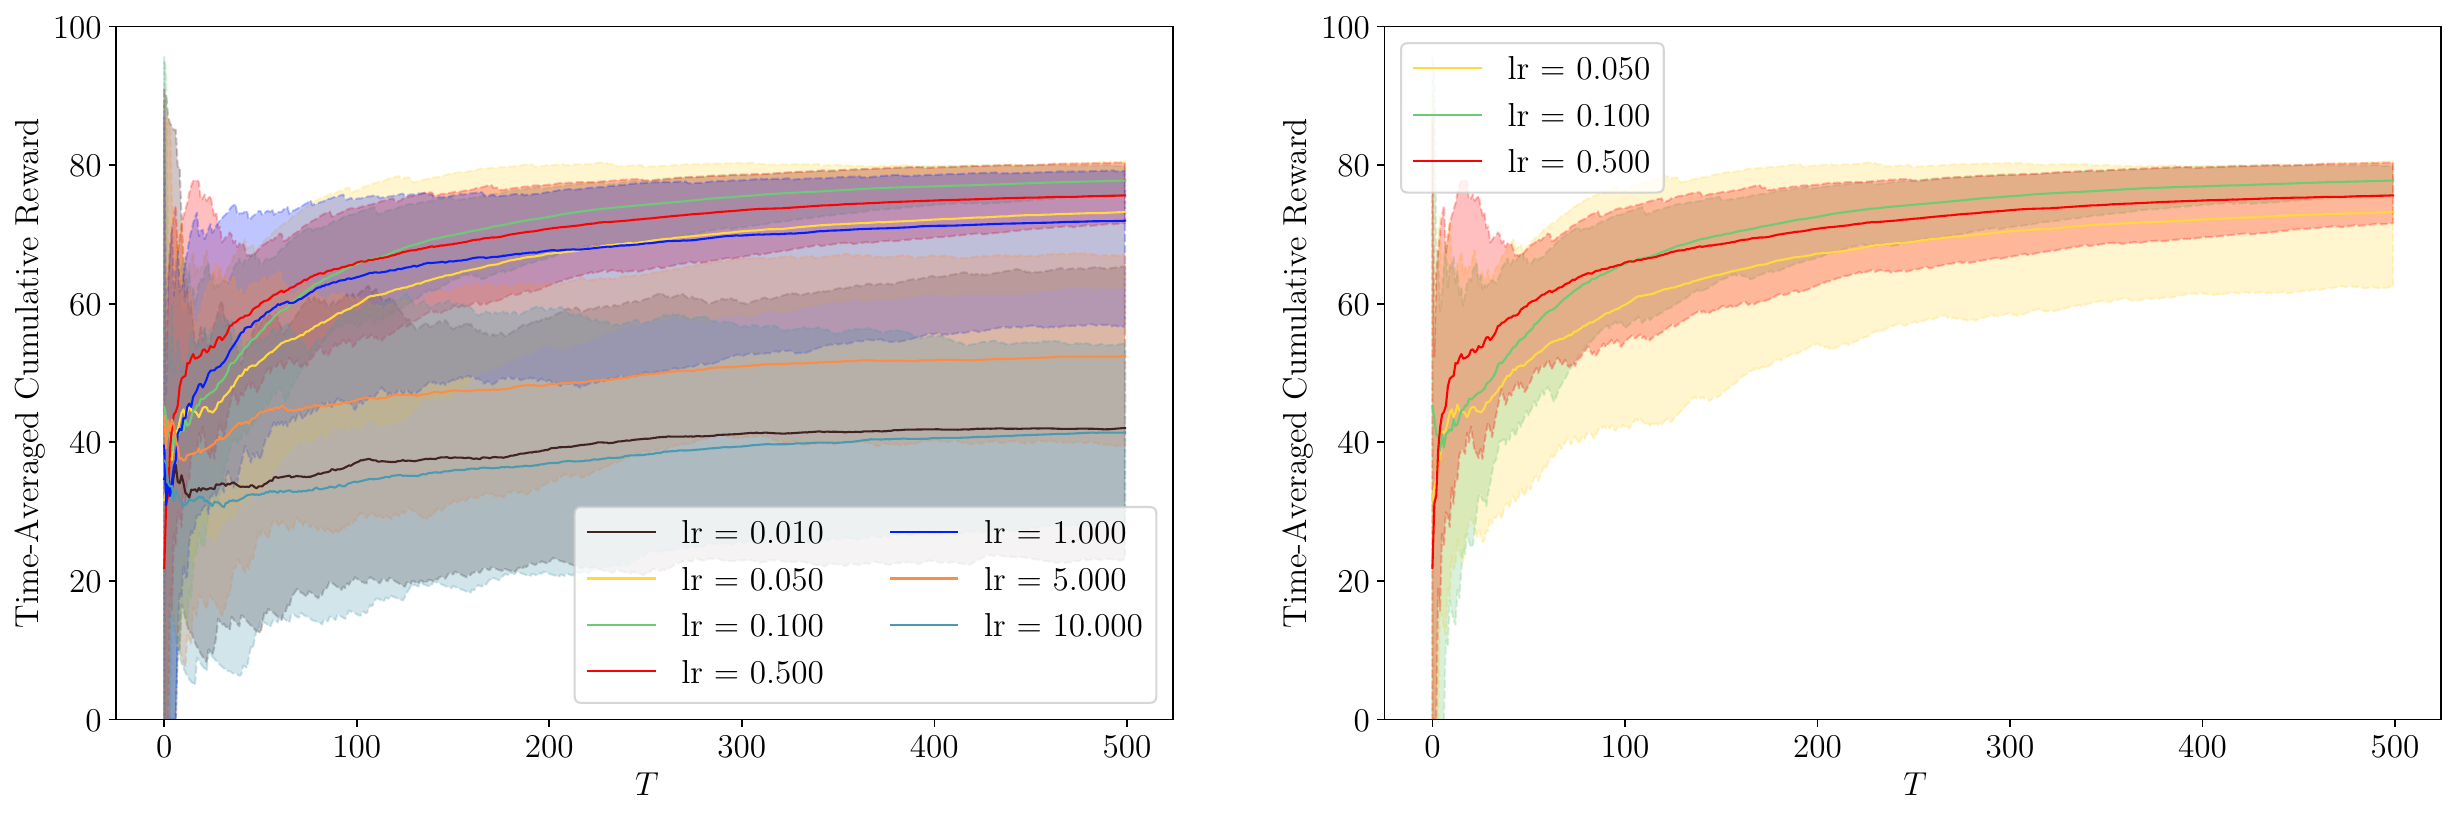}
    \caption{Time-averaged cumulative reward for \texttt{DFL} with different learning rate. Results are computed from 20 trials with a horizon $T = 500$.}\label{fig:sup2}
\end{figure*}

\newpage
\bibliographystyle{apalike}
\bibliography{supref}
\end{document}
